# Supplementary material for: Behind the Veil: Enhanced Indoor 3D Scene Reconstruction with Occluded Surfaces Completion
Source: arXiv:2404.03070 source file (2024-04-03)
Supplement: Supplementary file 1 [file 6_suppl.tex]

%\clearpage
% \setcounter{page}{1}
% \maketitlesupplementary
In this appendix, we provide more details on the datasets, evaluation metrics, and baselines in Appendices~\ref{subsection1}, \ref{subsection2}, and \ref{subsection3}. 
Additionally, we elaborate on our method implementation, including data preparation, network designs and training in Appendix~\ref{subsection4}.
%Moreover, we present comparison evaluation results on the ICL-NUIM~\cite{handa} dataset in Appendix~\ref{subsection5}. 
Furthermore, the runtime analysis and video demo are provided in Appendices~\ref{subsection6} and \ref{subsection7}, respectively.
Lastly, we include further information about our newly developed 3D Complete Room Scene (3D-CRS) dataset in Appendix~\ref{subsection8}.

% More comparison visualizations on the iTHOR~\cite{ai2thor} dataset are presented in Appendix~\ref{subsection2}.
% We also provide the visual comparison of room layout after furniture removal on 3D-CRS dataset in Appendix~\ref{subsection2}. 
% We include an additional ablations study to analyse the impact of the training scene numbers and depth sample numbers in Appendix~\ref{subsection3}.

\section{Datasets}
\label{subsection1}
We evaluate the proposed method with the baselines on two datasets: 3D-CRS and iTHOR scene dataset from AI2-THOR~\cite{ai2thor}.
%While the Geo-decoder training only requires a sequence of depth images, the 3D Inpainter training necessitates complete 3D scene meshes where the invisible surfaces are provided. 
Most of the existing public indoor RGB-D datasets don't provide the completed 3D meshes of room scenes.
To validate the generalization of our approach, we created a new dataset named 3D Complete Room Scene (3D-CRS) using Unreal Engine 4.27 for the main experiment.
3D-CRS contains 20 distinct indoor room scenes, each with RGB, depth, normal, semantic/instance masks, and camera trajectories.
Notably, we provide the completed 3D scene meshes for each room, consisting of both 3D furniture meshes and room layout meshes. 
We are capable of generating an infinite amount of data from the 3D complete scene mesh, by using a virtual camera in Unreal Engine.
For the experiments conducted in this paper, we only utilized depth images and 3D room meshes.
%We plan to release the 3D-CRS dataset to the public, provided that there are no conflicts with commercial interests in the future.
%
We further employ the iTHOR dataset as the complementary experiment, which provides the complete 3D scene meshes.
% It contains a collection of 13 high-quality, photorealistic indoor scenarios. 
% These environments encompass different rooms typical in a household, such as kitchens, bathrooms, living rooms, and bedrooms.   
%One of the key features of  iTHOR-AI2-THOR is that an AI agent can interact with objects in these environments in a multitude of ways.
iTHOR is a near photo-realistic interactable framework for embodied AI agents, including 120 room-scale scenes manually modelled by 3D artists. 
From this collection, we selected 13 living room models and exported their scene meshes by Unity for our second experiment.  
% For each scene, we crafted a camera trajectory by interpolating an elliptical spline and introducing random deviations to each camera pose. 
% In each room, we generated 100 distinct camera poses. 
%Using the Trimesh~\cite{trimesh} raytracer, we then obtained depth frames corresponding to each of these poses.
%We include more details on 3D-CRS dataset building, data preparation and network implementation in the Supplementary Material.

%
\begin{figure}[h]
\centering
\includegraphics[width=1.0\columnwidth]{figures/network_details_new.pdf}
\vspace{-3mm}
\caption{Network Architecture of Geo-decoder and 3D Inpainter}
\label{fig:main:network_details}
\vspace{-3mm}
\end{figure}

\section{Metrics}
\label{subsection2}
Following the evaluation metrics in BNV-Fusion~\cite{li2022bnv}, the standard metrics Accuracy~(Accu.), Completeness~(Comp.) and F1 score~(F1) are employed for the quantitative analysis. 
To be specific, we firstly uniformly sample 100,0000 points from the ground truth completed 3D meshes and generated 3D meshes, respectively, then compute  the Accu., Comp. and F1 metrics.
Accu. calculates the fraction of points from the reconstructed 3D mesh which is closer to points from the ground truth completed 3D mesh than a threshold distance of 2.5cm.
Similarly, Comp. calculates the fraction of points from the ground-truth completed 3D mesh which is closer to points from the reconstructed 3D mesh than a threshold distance of 2.5cm.
The overall performance metric, F1, is defined as the harmonic mean of Accu. and Comp. 

\section{Baselines}
\label{subsection3}
In our comparison experiments, we aimed to demonstrate the accuracy of our proposed method by comparing it against three baseline methods: TSDF-Fusion~\cite{Zhou2018}, Go-Surf~\cite{wang2022go-surf} and BNV-Fusion~\cite{li2022bnv}. 
TSDF-Fusion~\cite{Zhou2018}, which is implemented in the Open3D library, is currently the SOTA explicit geometry-based 3D surface reconstruction method.
BNV-Fusion~\cite{li2022bnv}, which utilizes neural implicit representations, is currently the SOTA implicit-style 3D surface reconstruction method.
For a fair comparison with the baseline Go-Surf~\cite{wang2022go-surf}, we modified its architecture by omitting the RGB branch during both the training and inference phases.
All the baselines, the same as our method, use only depth images as input, ensuring a fair basis for comparison.
It's important to note that the encoder used in BNV-Fusion is pre-trained on the large-scale ShapeNet dataset, notably improving the accuracy of visible surface reconstruction.
However, our method does not involve this particular pre-training step.

%BNV-Fusion method~\cite{li2022bnv}, which utilizes neural implicit representations, has achieved state-of-the-art performance on the 3D surface reconstruction benchmark.
%To ensure a fair comparison, all competing learning-based methods utilized only depth images and associated camera poses during training and inference. 
%

\section{Implementation Details}
\label{subsection4}

\textbf{Data Preprocessing}:

\textbf{1) Mesh Processing}: 
It was noted that human-created meshes frequently have artifacts on the exteriors of room layouts. 
To maintain consistency and purity in our ground truth meshes, we manually culled these unwanted external structures. 
Once these meshes were culled, we further processed them to be watertight using~\cite{huang2018robust}, enabling the computation of Signed Distance Functions (SDF).

\textbf{2) Depth Image Rendering}: 
For each scene, we first generate the camera trajectories. 
These trajectories are defined through Catmull-Rom spline interpolation, anchored on a series of manually chosen control points. 
Using the Trimesh raytracer~\cite{trimesh}, we render depth images corresponding to each camera pose. 
The number of sampled depth frames in each scene of 3D-CRS and iTHOR dataset are given in Table~\ref{tab:table6} and Table~\ref{tab:table7} respectively. 
The depth images for both datasets are rendered at a resolution of $1024 \times 768$.
% For 3D-CRS dataset, we define the trajectory by a. 
% For iTHOR dataset, we craft a trajectory by interpolating an elliptical spline and introducing random deviations to each camera pose. 

\textbf{3) Point Sampling}: 
% To prepare the training data for our 3D Inpainter, we extract SDF samples from each training scene. 
% Each mesh is first normalized, followed by sampling around $8\times 10^{6}$ signed distances close to the surface and an equal number of negative signed distances uniformly distributed 
% inside the furnitures.
% For near-surface samples, we maintain a 50\% ratio between visible and invisible areas. 
% The negative samples, representing the interior of objects, are considered as invisible areas. 
% Additionally, Gaussian noise is applied to the surface points to mimic the noise in depth measurements.
To prepare the training data for our 3D Inpainter, we extract SDF samples from each training scene. 
Each mesh is first normalized, followed by sampling around $8\times 10^{6}$ signed distances close to the surface and an equal number of signed distances uniformly distributed within the scene bounding box.
For non-surface samples, we maintain a 50\% ratio between positive and negative SDFs, representing visible free space and invisible interior of furniture, respectively. 

\textbf{Octree Feature Volume:} 
The voxel resolution in our configuration is set to 2 cm, and the latent code assigned to each corner of the octree node is set to 12 dimension.

\textbf{Network Architecture}: 
Figure~\ref{fig:main:network_details} illustrates the network architecture of the Geo-Decoder and 3D Inpainter. 
The Geo-Decoder employs a relatively shallow multilayer perceptron (MLP) consisting of 4 fully connected layers. 
Each of these layers is followed by a ReLU activation, except for the final layer. 
In contrast, the 3D Inpainter utilizes a network structure similar to DeepSDF~\cite{park2019deepsdf}, consisting of 8 fully connected layers. 
These layers are applied with weight normalization and interconnected via ReLU activations and a 0.3 dropout rate, except for the last layer. 
A skip connection is integrated at the 4th layer of the 3D Inpainter.

\textbf{3D Inpainter Training:}
In the training phase of the 3D Inpainter, our approach starts with randomly selecting a scene, loading its octree feature volume along with training samples, and then optimizing both the features and the 3D Inpainter over several consecutive iterations. 
Subsequently, we save the feature volume and repeat this process for each scene until all scenes have been trained within an epoch.
We experimentally found that 100 consecutive iterations per scene produces a desirable balance between generalization across different scenes and accuracy within a specific scene. 
The 3D Inpainter is offline trained using Adam optimizer with a learning rate of 1e-3.
The training of our 3D Inpainter is conducted on an NVIDIA RTX 3090 GPU for 100 epochs, which takes about 8 hours.

\textbf{Geo-decoder Optimization:}
The Geo-decoder is online optimized using Adam optimizer with a learning rate of 1e-2. 
The optimization process is conducted on an NVIDIA RTX 3090 GPU for 1000-10000 iterations, which approximately takes 3-30 mintues.
The number of iterations can be chosen based on different application requirements, which is a trade-off between speed and accuracy.

\textbf{Octree Feature Training and Optimization:}
During both offline training and online optimization, we observed that high-level features in the octree have less fluctuation and faster convergence during training, in contrast to low-level features. 
Therefore, we implemented a learning rate decay approach for octree features, progressively reducing the learning rate from high to low levels. This decay starts from an initial rate of 1e-3 and decreases for each level at a rate of 0.5.

\textbf{3D Surface Generation:} 
Our method is capable of inferring SDFs at arbitrary 3D locations. 
For the extraction of triangle meshes, we use Marching Cubes~\cite{lorensen1987marching}, applying a spatial resolution of 1cm.

\begin{table}[t]
\centering
\begin{tabular}{cccccc}
\hline
\textit{Scene} & \textit{01} & \textit{02} & \textit{03} & \textit{04} & \textit{05} \\ 
Depth Frames    & 199 & 172 & 188 & 235 & 156 \\
\hline
\textit{Scene}& \textit{06} & \textit{07} &\textit{ 08} & \textit{09 }& \textit{10} \\ 
Depth Frames    & 235 & 223 & 240 & 176 & 121 \\
\hline
\textit{Scene}& \textit{11} & \textit{12} & \textit{13} & \textit{14} &\textit{ 15} \\ 
Depth Frames     & 275 & 110 & 243 & 199 & 200 \\
\hline
\textit{Scene} & \textit{16} & \textit{17} & \textit{18} &\textit{ 19 }& \textit{20} \\ 
Depth Frames     & 155 & 210 & 200 & 187 & 278 \\
\hline
\end{tabular}
\vspace{-3mm}
\caption{The number of depth images sampled from each scene in the 3D-CRS dataset.}
\label{tab:table6}
\vspace{-3mm}
\end{table}
\begin{table}[t]
\centering
\begin{tabular}{cccccc}
\hline
\textit{FloorPlan}  & \textit{202} & \textit{205} & \textit{206} & \textit{207} & \textit{210} \\ 
Depth Frames    & 100 & 100 & 100 & 100 & 100 \\
\hline
\textit{FloorPlan}   & \textit{213} & \textit{217} & \textit{219} & \textit{220} & \textit{225} \\ 
Depth Frames     & 100 & 100 & 100 & 100 & 100 \\
\hline
\textit{FloorPlan}   & \textit{226} & \textit{228} & \textit{229} &  &  \\ 
Depth Frames    & 100 & 100 & 100 &  &  \\
\hline
\end{tabular}
\vspace{-3mm}
\caption{The number of depth images sampled from each scene in the iTHOR dataset.}
\label{tab:table7}
\vspace{-3mm}
\end{table}

\section{Runtime Analysis}
\label{subsection6}
The network is implemented under the PyTorch framework and is tested on a machine equipped with an NVIDIA RTX 3090 GPU accelerated by CUDA and cuDNN.
The inference runtime of our framework can be mainly divided into two distinct steps: 1) the octree feature volume building costs around 0.2 second per depth frame with $1024 \times 768$ resolution; 2) the Geo-decoder and feature optimization takes about 0.2 second per iteration. 
The number of iterations can vary between 1000 to 10000, allowing flexibility to balance speed and accuracy based on the specific application requirements.

% Secondly, the Geo-decoder optimization and 3Dtakes 
% Thirdly, the 3D Inpainter generate the occluded SDFs using
% Note that steps 2 and 3 is executed simultaneously, in parallel.
% Mesh extraction is excluded from the runtime calculation as it runs on a separate thread.
%Overall, our proposed method achieves a frame rate of nearly XXX frames per second (fps) on an NVIDIA RTX 3090 GPU, which is comparable to the BNV-Fusion method.

\section{Video Demo}
\label{subsection7}
%Due to the file size limit, we have only attached a concise video demo of one scene from the 3D-CRS dataset. 
We attach a video demo of visual comparison results in one scene.
%from the 3D-CRS dataset.
The video showcases the 3D surface reconstruction of the scene using our method, as well as the BNF-Fusion and TSDF-Fusion methods, along with the ground truth, while following a virtual camera trajectory.
